# Supplementary material for: Spot-On: A Mixed Reality Interface for Multi-Robot Cooperation
Source: arXiv:2505.22539 source file (2025-05-28)
Supplement: Supplementary file 1 [file X_suppl.tex]

\clearpage
\setcounter{page}{1}
\maketitlesupplementary
